# Supplementary material for: Reactive Multi-Robot Navigation in Outdoor Environments Through Uncertainty-Aware Active Learning of Human Preference Landscape
Source: arXiv:2409.16577 source file (2024-09-25)
Supplement: Supplementary file 1 [file supplementary.tex]

\title{\LARGE \bf Supplementary Materials
}

\textbf{Preliminaries}: In the ubiquitous robot system with $n$ robots, the position of each robot $i \in I=\{1,...,n\} \subset N$ is denoted by $r_i \in R^3$. To be simplified, all robots used in this work are considered to have the same dynamic model and non-rotating cube shape. The volume of robots is denoted as $V \subset R^3$. Let $W$ be the workspace of the multi-robot system and the environment it is acting in. The collision-free workspace is given by $W = R^3 \setminus (O+V)$, where the volume of obstacle set $O$ is dilated by the volume of robots $V$. The safety collision-free workspace is given by $W = R^3 \setminus (O+V+safety_{distance})$, where $safety_{distance}$ represents the minimal distance between the robot and obstacles that are human-acceptable.

\subsection{Human preference and MRS flocking}
In this work, human preferences are mainly specified by \textit{"Progress", "Quality" and "Safety"}. \textit{"Progress"} represents mission efficiency, which is mainly affected by "covering area", "flying speed", and "team formation". An MRS flocking with a big covering area, sparse team formation, and high flying speed can quickly complete search tasks; \textit{"Quality"} denotes task effectiveness, which is affected by "flying height" and "flying speed". The higher the flying height/speed is, the less likely it is for an MRS to discover a target. \textit{"Safety"} refers to the collision aspect when drones are used in the workplace and are affected by \textit{"safety distance"}. In an open environment, humans prefer to complete tasks quickly, pay more attention to task progress, and pay less attention to task quality and system security. While in a cluttered environment, humans prefer to be cautious about robot operation by maintaining robot safety and task quality. %Figure \ref{beha} shows details of expected robot behavior corresponding to three specific environment types.

The human preference-based multi-robot flocking process is considered to be parameterized by human preference over a set of flocking parameters. Let $\{h_{inner}, h_{height}, h_{speed}, h_{safety}, h_{formation}\}$ be the set of flocking parameters, which can be used to represent and explain human preference $H$. $h_{inner}$ denotes the minimal distance between robots; $h_{height}$ denotes the flying height of the robot system; $h_{speed}$ represents the flying speed of the multi-robot system; $h_{safety}$ represents the minimal distance between robots and obstacles; and $h_{formation}$ denotes coordination pattern or arrangement that MRS can accomplish through the use of advanced control algorithms.

In \cite{vasarhelyi2018optimized}, the author designed a tunable self-propelled flocking model, which can guarantee more stable behavior under the conditions of larger flocking speeds and also in confined spaces. In this work, we extended the flocking method by involving human preference.  In the subsections below, we present the exact mathematical formulation of our human preference based multi-robot flocking model.

\subsubsection{flocking speed}
Given robot's desired position $r_{goal} \in R^3$ and current $i$'s position $r_{i} \in R^3$, robot $i$ should flock in the goal direction with human preferred speed $h_{speed}$.
\begin{equation}
    v_{i}^{flock} = \begin{cases} \frac{r_{goal} - r_{i}}{|r_{goal} - r_{i}|}h_{speed} & if(|r_{goal} - r_{i}| > 0.2) \\ \frac{r_{goal} - r_{i}}{|r_{goal} - r_{i}|+0.4}h_{speed} & otherwise\end{cases}
\end{equation}

\subsubsection{repulsion}
A simple half-spring model was used for local repulsion, which is a linear distance-dependent central velocity term with a cutoff at a maximum interaction range:
\begin{equation}
    v_{ij}^{rep} = \begin{cases} (h_{inner} - r_{ij})\frac{r_i - r_j}{r_{ij}} & if(r_{ij} \leq h_{inner}) \\ 0 & otherwise\end{cases}
\end{equation}
where $r_{ij}=|r_i - r_j|$ denotes the distance between robot $i$ and $j$. The total repulsion term calculated for robot $i$ is \begin{math} v_{i}^{rep} = \sum_{j \neq i}v_{ij}^{rep} \end{math}.

\subsubsection{attraction}
For local attraction, the mechanism used is similar to local repulsion:
\begin{equation}
    v_{ij}^{att} = \begin{cases} (r_{ij} - h_{inner})\frac{r_j - r_i}{r_{ij}} & if(r_{ij} \ge h_{inner}+0.1) \\ 0 & otherwise\end{cases}
\end{equation}
The total attraction term calculated for robot $i$ with respect to the other robots is \begin{math} v_{i}^{att} = \sum_{j \neq i}v_{ij}^{att} \end{math}.

\subsubsection{interaction with obstacles}
Compared to the repulsion mechanism, we still choose a simple half-spring model. But instead of a linear distance-dependent central velocity term, we have used a constant velocity term with a cutoff at a maximum distance based on human-preferred safety distance to obstacles, $h_{safety}$, under which robots start to adjust its velocity to get away:
\begin{equation}
    v_{ij}^{saf} = \begin{cases} h_{speed}J & if(d_{ij} \leq h_{safety}) \\ 0 & otherwise\end{cases}
\end{equation}
In the above equation, $d_{ij}$ denotes the distance between robot $i$ and obstacle $j$. $J$ denotes an indicator function representing which direction the robot should run away. The total safety term calculated for robot $i$ with respect to the obstacles is \begin{math} v_{i}^{saf} = \sum_{j}v_{ij}^{saf} \end{math}.

\subsubsection{flying height}
Similar to "interaction with obstacles", we have used a constant velocity term with a cutoff at a minimum distance based on human preferred flying height, 1.0, above which robots start to adjust their velocity:
\begin{equation}
    v_{i}^{hei} = \begin{cases} h_{speed}J & if(dis \ge 0.2) \\ \frac{r_i^{height} - h_{height}}{dis+0.4}h_{speed} & otherwise\end{cases}
\end{equation}
In the above equation, $dis = |r_i^{height} - h_{height}|$; $J$ denotes an indicator function. If the current flying height is lower than human preference, $J$ will denote the increase in robot $i$'s flying height. And if the current flying height is higher than human preference, $J$ will denote the decrease robot $i$'s flying height.

\subsubsection{formation}
In a specific MRS formation $h_{formation}$, with robot $i$'s desire position $h_{formation}^i$ and its current position $r_i$, a simple string model is used:
\begin{equation}
    v_{i}^{fmt} = \begin{cases} \frac{h_{formation}^i - r_{i}}{dis}h_{speed} & if(dis > 0.1) \\ \frac{h_{formation}^i - r_{i}}{dis+0.2}h_{speed} & otherwise\end{cases}
\end{equation}
where $dis=|h_{formation}^i - r_{i}|$.

\subsubsection{velocity alignment}
Pairwise velocity alignment can be obtained with a velocity term that depends on the difference of the velocity vectors and the distances of nearby robots.
\begin{equation}
    v_{ij}^{ali} =  [2.0,2.0,1.0]\frac{v_i - v_j}{(r_{ij}+1.0)^2}
\end{equation}
The total velocity alignment term calculated for robot $i$ with respect to the robots is \begin{math} v_{i}^{ali} = \sum_{j \neq i}v_{ij}^{ali} \end{math}.

To calculate the desired velocity, we take the vectorial sum of all the
interaction terms introduced before:

    \begin{multline} v_i = 0.3v_i^{flock} + 0.35v_i^{fmt} + 0.35v_i^{rep} \\+ 0.35v_i^{att} + 0.4v_i^{saf} + 0.2v_i^{hei} + 0.1v_i^{ali} \end{multline}

After this superposition, we also introduced a cutoff based on human-preferred flying speed, keeping the direction of the desired velocity but reducing its magnitude if it is over the limit:
\begin{equation}
    v_i = \frac{v_i}{\| v_i \|}h_{speed}
\end{equation}

\subsection{Raw features and data pre-process}
In this paper, multiple diverse proprioceptive and exteroceptive sensors were used to improve environment representations by collecting heterogeneous data. As for the exteroceptive sensor, a RGB camera was mounted on each drone, allowing for a wide range of perspectives of unstructured environments in front of the robot. Lidar was also applied to measure drone distances and create a 3D model of the surrounding environment with a frame rate of 30 Hz. As for proprioceptive sensors, motor speed, inertial measurement unit (IMU) measurement, and power consumption were also used to measure the drone's internal status. All of these collected data were used together as input for evaluating and comparing outdoor environment adaptation methods.

Then, commonly used environment features can be extracted from the multi-sensory data collected by robot sensors. As for exteroceptive data from the RGB camera, a trained neural network model was used to compute visual features of the outdoor environment from color images. The neural network (3 convolution layers, 3 max-pooling layers, 1 dropout layer, and 1 fully connected layer) was first trained to classify collected images into different environment types. Then the features calculated from the last layer were used as extracted features. Therefore, the extracted features can capture different visual characteristics of the environments. Additionally, the point cloud data collected by the lidar sensor is used to compute 3D map based on grids to discretely represent the unstructured surrounding environment. 3D maps are utilized to calculate the distance between drones and obstacles. Besides, the size of obstacle-free areas (height, width, and length) is also calculated. At last, data from proprioceptive sensors are combined with the extracted visual and lidar features to form an input vector that is used to represent unstructured environments.

\subsection{Optimization-based MRS behavior adjustment}

In this work, we extended the flocking method proposed in \cite{vasarhelyi2018optimized} by involving obstacle-free largest convex region searching and optimization-based MRS behavior planning, which can guarantee stable and safe robot behaviors in unstructured environments.

\textbf{Obstacle-free largest convex region searching}: To compute the largest convex region of obstacle-free space, iterative regional inflation by semi-definite programming method (IRIS) was designed in [27]. In the proposed method, two convex optimizations are used: (1) given the workspace $W$ and obstacles $O$, a set of hyperplanes is generated and optimized to build an obstacle-free convex region $P$; (2) with the calculated obstacle-free space $P$, find the maximum-volume ellipsoid $\Xi$ inside $P$ through the semi-definite program. Both the hyperplanes and the ellipsoid are refined over
several iterations to obtain a large obstacle-free convex region.

The ellipsoid is represented as an image of the unit ball: $\Xi(C,d)=\{x=C\tilde{x}+d; \|\tilde{x}\| \le1\}$. The set of hyperplanes is represented as linear constraints: $P=\{x;Ax\le b\}$. Given that the volume of $\Xi$ is proportional to the log of the determinant of $C$, the volume of $\Xi$ can be efficiently maximized since the log of the determinant of $C$ is a concave function. At last, the goal is to solve the following non-convex optimization problem: 
\begin{align}
    \max_{A,b,C,d} &\quad logdet(C) \\
    \text{s.t.} &\quad a_j^Tv_k \ge b_j; \quad v_k \in O \\
    &\quad \sup_{\|\tilde{x}\|\le1}a_i^T(C\tilde{x}+d) \le b_i
\end{align}
where $a_j$ denotes the row of $A$, $b_j$ represents the element in $b$. $v_k$ are points in obstacle $O$. Instead of solving this optimization problem directly, the algorithm alternates between searching for the hyperplanes $P$ and optimizing
for the largest $\Xi$ inside $P$. For the detailed outline of IRIS, please refer to [27].

\textbf{Optimization-based safe MRS behavior planning}: Given that the learned human preference model may not generalize well to the current environment, the predicted human preference values may be inaccurate or have high variance. If we directly apply the predicted human preference values $\hat{H}$ to MRS, the security of MRS will be greatly challenged. For example, MRS may fly very close to an obstacle and collide with it when there is a wind disturbance to obtain robust and safe MRS flocking behavior, we designed an optimization-based MRS behavior planning mechanism, which can ensure the safety of MRS even with inaccurate predicted human preference values.

From the "Obstacle-free largest convex region searching" step, a set of hyperplanes represented as linear constrains: $P=\{x; Ax\le b\}$ can be obtained. Given the volume of drone $V$ and predicted safety distance between drone and obstacles $h_{safety}$,  the hyperplanes are dilated to $P'=\{x; Ax\le B\}$. Given predicted human preference $\hat{H}$, goal position $r_{goal}$, and current hyperplanes $P'$, the goal of "Optimization-based safe MRS behavior planning" is to find a set of optimal transform parameters of $\hat{H}$ to ensure the safety of MRS. For example, the internal distance between drones is adjusted according to the predicted MRS formation and $P'$, and if the predicted formation is not suitable for the current situation, another suitable formation is selected from a finite set of formations. The optimization problem can be formatted as:
\begin{align}
    \max_{t,s,R} &\quad \|r_{goal}-(t + Rsx_c)\|^2_2 + w_1\|s - \hat{h}_{inner}\|^2_2 \\
    & \quad \quad + w_2\|[0,0,1](t + Rsx_c) - \hat{h}_{height}\|^2_2 \\
    \text{s.t.} &\quad a_j^T(t + Rsx_i) \ge B_j
\end{align}
where $t \in R^3$ is translation vector; $s \in R^1$ represents scale parameter; $R \in R^{3 \times 3}$ denotes rotation matrix; $x_c$ denotes the center point of predicted MRS formation; $x_i$ represents drone $i$'s position in the predicted MRS formation; $a_j$ denotes the row of $A$; $B_j$ represents the element in $B$.

As for the predicted MRS formation, if there exists an optimal solution. The obtained transformation parameters $t^*,s^*$ and $R^*$ will be used to calculate the goal position of each robot and adjust predicted human preference $\hat{H}$. However, if there is no suitable solution, we will try to find a solution for all the formations in the provided finite set of formations and choose the formation and corresponding optimal transformation parameters with minimal loss as the current solution. Then we can calculate the goal position of each robot and adjust the predicted human preference. With the goal position and adjusted human preference, we then can control MRS by using the Human preference-based MRS flocking method.
